# Supplementary material for: GeoReF: Geometric Alignment Across Shape Variation for Category-level Object Pose Refinement
Source: arXiv:2404.11139 source file (2024-04-17)
Supplement: Supplementary file 2 [file M2.tex]

\begin{figure}[htbp]
\centering
% \vspace{-2mm}
\includegraphics[width=1\linewidth]{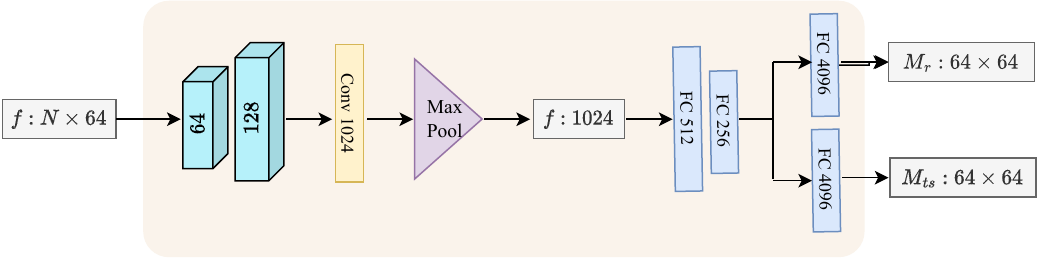}
\caption{\footnotesize \textbf{Structure of Matrix Net that outputs $M_{r}$ and $M_{ts}$} } 
\label{fig:M2}
\end{figure}
